# Supplementary material for: Diffusion Model is a Good Pose Estimator from 3D RF-Vision
Source: arXiv:2403.16198 source file (2024-07-22)
Supplement: Supplementary file 1 [file X_suppl.tex]

\setcounter{section}{0}

\section*{Appendix}

\section{mmWave Human Sensing}
In Figure~\ref{sensing}, we illustrate the utilization of mmWave radar for human sensing, which detects human actions within a range of 3-5 meters from the radar. This process generates mmWave point clouds (PCs). Simultaneously, a keypoint annotation system such as VICON, Mocap, or Cameras is deployed to record ground-truth human poses for reference. The mmWave radar-based human pose estimation refers to training a neural network to estimate human poses using mmWave radar point clouds as input.

For general mmWave human sensing, FMCW (Frequency Modulated Continuous Wave) chirp signals are transmitted and their reflections are received through antenna arrays. These chirp signals are defined by parameters such as start frequency $f_c$, bandwidth $B$, and duration $T_c$. To generate radar PCs~\cite{xue2021mmmesh}, range-FFT separates different frequency components $f$ from the IF signals, enabling the extraction of object distances using the formula $R=\frac{cfT_c}{2B}$, where $c$ is the speed of light. Doppler-FFT measures phase changes $\omega$ of the IF signals, facilitating the calculation of object velocities using $v=\frac{\lambda\omega}{4\pi T_c}$, where $\lambda$ is the wavelength of the chirp. Elevation angles $\varphi$ and azimuth angles $\theta$ of the detected objects are determined based on $\varphi=sin^{-1}(\frac{\omega_z}{\pi})$ and $\theta=sin^{-1}(\frac{\omega_x}{cos(\varphi)\pi})$, where $\omega_x$ is the phase change between azimuth antennas and corresponding elevation antennas, and $\omega_z$ is the phase change of consecutive azimuth antennas. Finally, the Cartesian coordinates (x, y, z) of the detected point clouds are calculated as follows: $x=R cos(\varphi) sin(\theta)$, $z=R sin(\varphi)$, and $y=(R^2-x^2-z^2)$.

\begin{figure}[!ht]
\centering
\includegraphics[width=3.0in]{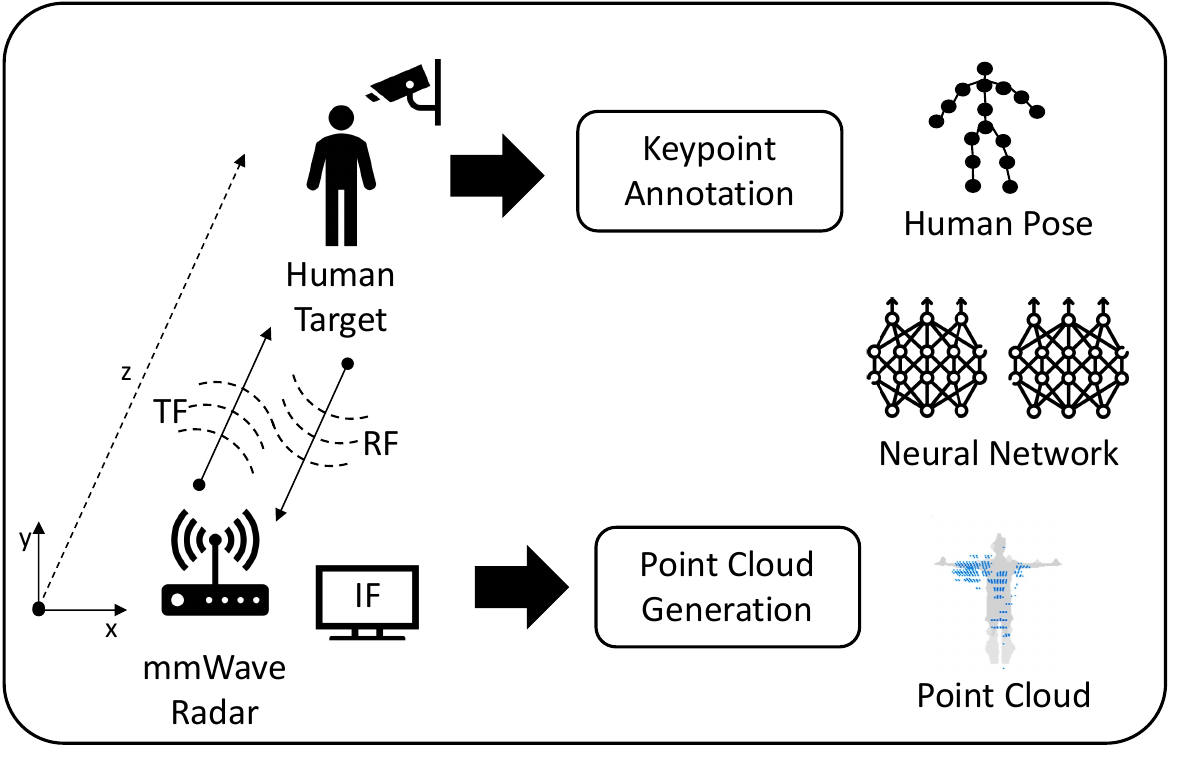}
\caption{Workflow of mmWave sensing and mmWave human pose estimation.}
\label{sensing}
\end{figure}

\section{The Diffusion Model for Human Pose Generation}
\label{mathdiff}
\subsubsection{Forward process.} The forward process involves the gradual sampling of increasingly noisy human poses, resulting in an intermediate distribution of noisy poses that serve as training guidance. Here, $k\in\left[1..K\right]$ denotes the diffusion steps, where noisy human poses $H_k$ are sampled by adding noise to the original ground truth pose $H_0$. Following the Markov process, we interatively add noise to the pose $H_{k-1}$ and obtain a noisier version of pose $H_k$: 
\begin{align}
q\left(H_k \mid H_{k-1}\right)&=\mathcal{N}\left(H_k \mid \sqrt{\alpha_k} H_{k-1},\left(1-\alpha_k\right) I\right), \\
H_k&=\sqrt{1-\beta_k} H_{k-1}+\beta_k \varepsilon,
\label{eq:sampling0}
\end{align} where $\beta_k$ denotes the noise scale, $\varepsilon \in \mathcal{N}(0,I)$ denotes the random noise, and $\alpha_k=1-\beta_k$. With a small noise scale $\beta_k \in [0.0001, 0.001]$, $H_k$ is approaching to $H_{k-1}$, which allows us to model both the forward sampling $q(H_{k}|H_{k-1})$ and the reverse estimation $p_\theta(\hat{H}_{k-1}|H_{k}, C)$ as Gaussian distributions. To directly sample $H_k$ from the ground truth $H_0$, Eq.~\ref{eq:sampling0} can be rewritten to: 
\begin{equation}
H_k=\sqrt{\gamma_k} H_0+\sqrt{1-\gamma_k} \boldsymbol{\varepsilon},
\label{diffusion_sample}
\end{equation}where $\gamma_k=\prod_{i \in[1 . . k]} \alpha_k$. Eventually, when $k\rightarrow\infty$, $H_k$ approaches pure random noise following Gaussian distribution. 

\subsubsection{Reverse process.} At each iteration $k$ of the reverse process, a cleaner pose $\hat{H}_{k-1}$ is estimated to approximate $H_{k-1}$ (generated by the forward process), given a noisy pose $H_k$ and the conditional set $C$. The reverse process can be formulated as:
\begin{equation}
p_\theta\left(\hat{H}_{0: K} \mid H_0, C\right)=p\left(H_K\right) \prod_{k=1}^K p_\theta\left(\hat{H}_{k-1} \mid H_k, C\right).
\end{equation}During training, $H_{1: K}$ are obtained by adding noise to the ground truth $H_0$, following the forward process. However, during inference, as the ground truth is unavailable, we set $H_{1: K} = \hat{H}_{1: K}$ by iteratively inputting the estimated human poses $\hat{H}_{1: K}$ into the trained diffusion model. As discussed in the main paper, $\hat{H}_K$ is initialized by a coarsely estimated pose $\Tilde{H}$ as the starting point of the reverse process.

\subsubsection{Model training.} We follow DDPM~\cite{ho2020denoising} for faster convergence of the diffusion model. Firstly, diffusion step $k\in\left[1..K\right]$ and $\varepsilon \in \mathcal{N}(0,I)$ are randomly sampled, and $H_k$ is calculated according to Eq.~\ref{diffusion_sample}. Then, the diffusion model is trained to approximate $\hat{\varepsilon}$ to $\varepsilon$, rather than directly approximate $\hat{H}_{k-1}$ to $H_{k-1}$. The learning objective following DDPM is formulated as: 
\begin{equation}
    \mathcal{L}_{\text {diff}}=\mathbb{E}_{k \sim[1, T]} \mathbb{E}_{\varepsilon \sim \mathcal{N}(0, I)}|| \varepsilon - \hat{\varepsilon}_\theta(H_k, k, C)\|^2_2 \\.
\label{eq:diff2-supp}
\end{equation}

\section{Evaluated Datasets}

\begin{table*}[!t]
\footnotesize
\centering
\caption{Overview of the datasets used for mmWave human pose estimation. }
\setlength{\belowcaptionskip}{0.2cm}
\resizebox{1.\textwidth}{!}{
  \fontsize{12}{14}\selectfont
\begin{tabular}{p{8em} p{11.5em} p{1em} p{16.5em} p{1em} p{13.5em}}
    \toprule
    \textbf{Dataset:} & \textbf{mmMesh} & & \textbf{mmBody} & & \textbf{mm-Fi} \\
    \midrule[1.5pt] \midrule
    \textbf{Radar Type:} & AWR1843BOOST mmWave radar from Texas Instruments. & & Phoenix mmWave radar from Arbe Robotics. & & IWR6843 60-64GHz mmWave radar from Texas Instruments. \\
    \midrule
    \textbf{Annotations:} & Mesh annotated by VICON motion capture system and generated by SMPL. & & 55 keypoints are annotated by the OptiTrack Mocap system; Mesh is generated by Mosh++ and SMPL-X. & & 2D keypoints are obtained by HRNet-w48 from two-view infra-red cameras; 3D keypoints are calculated by triangulation. \\
    \midrule
    \textbf{Point format:} & Cartesian: (x, y, z); PC attributes: (range, velocity, energy). & & Cartesian: (x, y, z); PC attributes: (velocity, amplitude, energy). & & Cartesian: (x, y, z); PC attributes: (velocity, intensity).\\
    \midrule
    \textbf{Public or not:} & No.  & & Yes. & & Yes. \\
    \midrule
    \textbf{\# of subjects:} & Not mentioned. & & 20 (10 males, 10 females). & & 40 (29 males and 11 females) \\
    \midrule
    \textbf{\# of actions:} & Not mentioned. & & 100 motions (16 static poses, 9 torso motions, 20 leg motions, 25 arm motions, 3 neck motions, 14 sports motions, 7 daily indoor motions, and 6 kitchen motions). & & 27 actions (14 daily activities and 13 rehabilitation exercises) for a duration of 30 seconds. \\
    \midrule
    \textbf{\# of frames:} & Not mentioned. & & 39892 frames for training and 28048 frames for testing. & & 133920 frames for training and 38400 frames for testing. \\
    \midrule
    \textbf{Scenes:} & Normal and occlusion. & & Lab1, Lab2, Furnished, Poor\_lighting, Rain, Smoke, and Occlusion.  & & Normal, Cross-subject, and Cross-environment. \\
    \bottomrule
    \end{tabular}
    }
    % \captionsetup{font=footnotesize}
    
    \label{tab:dataset}
\end{table*}%

As shown in Table~\ref{tab:dataset}, we present a comparison of existing datasets for point-cloud-based mmWave human pose estimation (HPE), focusing on several key attributes including mmWave radar sensor type, keypoint annotations, radar point cloud format, dataset size, and the variety of scenes covered in the dataset.

\subsubsection{mmMesh~\cite{xue2021mmmesh}.} mmMesh is the systematic work proposing mmWave human sensing (mesh reconstruction) with an off-the-shelf commercial mmWave sensor, AWR1843BOOST mmWave from Texas Instruments~\cite{rao2017introduction}. It provides a systematic way to annotate human mesh (including human keypoints) with the VICON system and SMPL~\cite{loper2023smpl} algorithm. The mmMesh dataset is presented for comparison, as it is not public and only contains normal and occlusion scenarios. 

\subsubsection{mmBody~\cite{chen2022mmbody}.} mmBody dataset is a public dataset for mesh reconstruction with multi-modal sensors: depth camera, RGB camera, and mmWave radar. Specifically,  Phonix mmWave radar from Arbe Robotics is chosen as the mmWave sensor, which extracts thousands of radar points for scene detection. Still, the detected radar point clouds are noisy and sparse compared to RGB and depth sensors. The dataset contains daily-life motions, with heterogeneous human motions including motion of the torso, leg, arm, etc. Due to numerous subtle limb motions in the dataset, it is challenging to accurately predict human poses. To evaluate the robustness of mmWave HPE, the dataset includes various cross-domain scenes (lab2 and furnished) and adverse scenes (dark, rain, smoke, and occlusion).  Meanwhile, except for lab2 containing seen subjects, all other scenes contain unseen subjects for testing, which is challenging for the model's generalizability. Our experiment is conducted following the mmBody settings~\cite{chen2022mmbody}.

\subsubsection{mm-Fi~\cite{yang2023mm}.} mm-Fi offers a broader scope of human sensing, including action recognition and HPE, leveraging a variety of multi-modal sensors: RGB(D), LIDAR, WiFi, and mmWave radar. It is a large-scale dataset with 40 subjects participating and over 15k frames for training and testing. The mmWave radar utilized in the dataset is IWR6843 60-64GHz mmWave, which is a low-cost option generating a limited number of radar points. The point cloud format omits redundant range features. Meanwhile, different from the other two datasets, the model is trained in a self-supervised manner, as the human pose annotations are obtained by RGB image using HRNet-w48~\cite{prabhakara2023high}. The annotations are rather unstable compared to the motion capture systems. To test the model's generalizability, the dataset also proposes the cross-subject and cross-environment splits. Our experiment follows protocol 1 (P1) to include all daily-life activities and adopt all splitting methods.

\section{Detailed Experiment Settings}

\subsection{Data Preprocessing}

\subsubsection{Radar point clouds preprocessing.} Due to radar sparsity and the occasional miss-detection, we follow \cite{an2022fast} to concatenate adjacent frames to enrich the number of points. Specifically, 4 frames are concatenated for mmBody and 5 frames are concatenated for mm-Fi. Further, since mmWave radar point clouds are generated by the targets with salient Doppler velocity, the number of radar points is frame-wise variant. As a result, to enable mini-batch training using PyTorch dataloader~\cite{paszke2019pytorch}, we perform zero-padding (null points with 0 values) to guarantee the invariant input tensor shape. For mmBody, we zero-padding the point clouds to 5000 points, while a dynamic padding technique~\cite{yang2023mm} is applied for mm-Fi. Moreover, to handle noisy radar points resulting from environmental reflection and interference, we perform point cloud cropping to select only the points within the region of human activities. For mmBody, the region of human activities is centered at the ground-truth pelvis location, with a region size of ($x$:$\pm 1.6$m, $y$:$\pm 1.6$m, $z$:$\pm 1.6$m). However, for mm-Fi, as point clouds are generated solely by moving targets, cropping is unnecessary.

\begin{figure}[!t]
\centering
\includegraphics[width=2.0in]{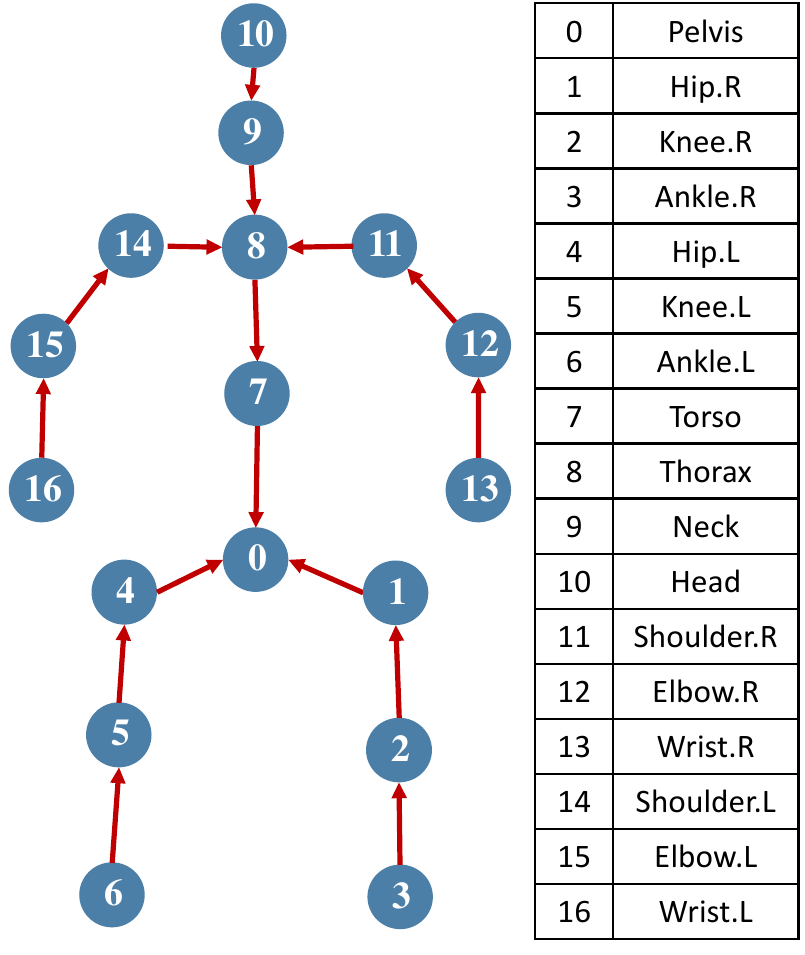}
\caption{Selected keypoints (ID and names) for mmWave human pose estimation. Red arrows indicate the select limbs.}
\label{pose}
\end{figure}

\subsubsection{Human pose and limb-length preprocessing.} Our ground truth keypoints $H=\{h_1,..,h_{17}\}$ are selected according to Figure~\ref{pose}. Following ~\cite{ionescu2013human3} to construct ground-truth human poses, we perform pose normalization by pelvis alignment: subtracting the pelvis position $h_1$ from every keypoint $h_{1:17}$ of the skeleton. It's worth noting that the pelvis alignment is missing for the mm-Fi dataset, resulting in a higher Mean Per Joint Position Error (MPJPE). Consequently, we incorporate human pose normalization for a fair comparison. To calculate the ground truth 16 limb-length $L=\{l_1,..,l_{16}\}$, we compute the $\mathcal{L}_2$ distance between two adjacent human keypoints, as selected according to Figure~\ref{pose}.

\subsection{Implementation of mmDiff}
% \subsubsection{Overall implementation.} 

% Our methods are trained for 100 epochs with a fixed batch size of 1024. The Adam algorithm~\cite{kingma2014adam} is used for optimization, with the learning rate set as $2e-5$, the gradient clip set to 1.0, and the momentum set to 0.9. The length of the forward/reverse diffusion process is set as $K=25$ with the constant $\beta$ sampling of 0.001. An average of 5 hypotheses is recorded for a fair comparison with non-diffusion methods. We choose Point4D~\cite{fan2021point} as the GRC's PC encoder for mmBody and PointTransformer~\cite{zhao2021point} for mm-Fi. We set $\Bar{K}=50$ for $\Bar{K}$NN algorithm for LRC, but due to insufficient radar points ($N<100$), the LRC module is neglected for mm-Fi. We further set $\Delta t = 8$ for TMC and $\lambda = 5$ for SLC. The hyper-parameters are obtained empirically, more precise hyper-parameter tuning tricks such as the Bayesian optimization could lead to better results. 

\subsubsection{Conditional diffusion model.} 
The GCN encoders, GCN blocks, and GCN decoders are designed following~\cite{zhao2022graformer} and~\cite{gong2023diffpose}. All MLPs are implemented as (LayerNorm, Linear, Dropout, ReLU, and Linear), and the temporal 1D-convolution extractor $g_2^{tem}$ is implemented as (Conv1D(k=3), Dropout, ReLU, Conv1D(k=3), MaxPool). The conditional diffusion model adopts a Graph Convolution Network (GCN) architecture inspired by GraphFormer~\cite{zhao2022graformer} as its backbone. The pose encoder and decoder utilize Chebyshev graph convolution layers~\cite{defferrard2016convolutional} to project human poses to 96-dimensional pose embeddings. The GCN block is implemented by stacking a Chebyshev graph convolution layer and a graph attention layer, with skip connection. The GCN backbone consists of 5 GCN blocks. Chebyshev graph convolution layer first projects the 96-dimensional pose embeddings to 96-dimensional hidden feature embeddings. Subsequently, each graph attention layer performs self-attention with 4 attention heads in a 96-dimensional hidden feature space. During training, the GCN backbone applies a dropout rate of 0.25 and an exponential moving average (EMA) rate of 0.999 0.999. The conditional embeddings are added at the start of each GCN block. Notably, as the Graph-Conditional Generation (GRC) model is trained before the diffusion training, the extracted conditional embeddings $C^{glo}$ require an additional projection to align with the human pose feature embeddings. This alignment is achieved through a Chebyshev graph convolution layer projecting from 64 dimensions to 96 dimensions.

\subsubsection{Radar point cloud encoder.} Since mmBody and mm-Fi utilize different mmWave radars for sensing, and mm-Fi has sparser point clouds, the design of the radar point cloud (PC) encoder within the Global Radar Context (GRC) model differs between the two datasets. For mmBody, the PC encoder adopts the point 4D convolution following the P4Transformer benchmark~\cite{fan2021point}. Anchors are selected using farthest point sampling (FPS) with a spatial stride of 32, resulting in the selection of 312 anchors. Ball query is then applied to retrieve nearby radar points within a radius of 0.1 and 32 samples. A temporal convolution with a kernel size of 32 and a stride of 2 is subsequently applied to encode the nearby PCs into a 1024-dimensional PC feature space. On the other hand, for mm-Fi, the radar PC encoder is designed following the PointTransformer approach~\cite{zhao2021point}. It utilizes 5 point-attention blocks with $n_{\text{neighbor}}=16$ and $d_f=128$ feature dimensions. After the radar PC feature encoders, the extracted PC features are concatenated with randomly initialized joint feature templates and fed into the global-transformer layers~\cite{vaswani2017attention}. 

\subsubsection{Global and local transformers.} 
The global transformer consists of $D = 10$ transformer layers, each utilizing $H=8$ attention heads and a hidden feature dimension of 256. The local lightweight transformer consists of $D=5$ transformer layers, $H=8$ attention heads, and a hidden feature dimension of 96. In each attention layer of both transformers, skip connections are applied. Additionally, after the local transformer, each anchor computes the proportion of points that are within a distance threshold of $thre=0.04$m. This proportion serves as a measure of reliability for the local features. We incorporate it by multiplying the local features with the calculated proportion (which falls in the range $[0,1]$). This approach helps to weigh the local features based on their distance to nearby points, enhancing the model's ability to focus on more relevant information.

\subsection{Implementation of other Compared Methods}
The methods using other modalities, e.g., RGB and depth are directly recorded from mmBody~\cite{chen2022mmbody}. Other methods use mmWave radar point clouds (PCs) as the input modality, which are described in detail:

\subsubsection{mmWave-based HPE methods.} 

For a more direct comparison of performance gains achieved by mmDiff, it's important to note that the radar point cloud (PC) encoders of P4Transformer~\cite{fan2021point} and PointTransformer~\cite{zhao2021point} are the same with mmDiff's radar PC encoder.

In the case of P4Transformer, which serves as the benchmark for mmBody, the PC encoder first utilizes a point4D convolution layer to extract PC features $F^{r} \in \mathbb{R}^{P \times 1024}$. Subsequently, a global transformer performs self-attention on these features. Unlike GRC modules, the input to the global transformer is solely the PC features $F^{r}$ without any joint feature templates $\Bar{F}^{j}$. Following the global transformer, a nonparametric max-pooling layer aggregates $\mathbb{R}^{P \times 1024}$ PC features into $\mathbb{R}^{1024}$. This aggregated feature is then dimensionally reduced into a $\mathbb{R}^{64}$ feature space through an MLP and decoded into $\mathbb{R}^{17*3}$ human poses. On the other hand, PointTransformer, which serves as the benchmark for mm-Fi, employs a point attention PC encoder to extract PC features. Similar to P4Transformer, a global transformer performs self-attention on these features. Then, a max-pooling layer aggregates PC features, followed by two MLPs for dimension reduction and pose decoding. Lastly, mmMesh~\cite{xue2021mmmesh} is implemented following its open-source design without modification.

\subsubsection{Camera-based 3D HPE methods.} 
Since camera-based 3D Human Pose Estimation (HPE) methods cannot directly utilize radar point clouds as input, we adopt a different approach. These methods typically involve pose-lifting, where 2D human poses are used as input to predict 3D human poses. Therefore, we fine-tune these models for 3D pose refinement: Given coarsely estimated 3D human poses $\Tilde{H}$, the models aim to estimate cleaner 3D human poses $\hat{H}$ by eliminating noise within $\Tilde{H}$. 

To ensure a fair comparison, the input coarse human poses $\Tilde{H}$ are the same for mmDiff and the compared 3D HPE methods. We implement PoseFormer~\cite{zheng20213d} following its open-source design. Similarly, we implement DiffPose~\cite{gong2023diffpose} using the same GCN diffusion backbone as used in mmDiff. This consistent setup allows for a direct comparison between the performance of mmDiff and these 3D HPE methods in refining 3D human poses.

\subsubsection{Other methods}
In this section, we provide a discussion of other mmWave-based methods that do not utilize PCs as the input modality, i.e. using raw radar signals or Range-Doppler (RD) maps. Specifically, Hupr~\cite{lee2023hupr}
 and MI-Mesh~\cite{ding2023mi} utilize raw radar signal to perform HPE. We summarize the difference between mmDiff with HuPR and MI-Mesh in Table~\ref{table:raw-compare}, regarding input modalities, evaluation dataset pros and cons, preprocessing methods, and reported joint errors. Quantitative comparisons are limited by the absence of datasets containing both RF raw data and radar PCs.

\begin{table}[!t]
\center
\resizebox{1.\linewidth}{!}{
    
    \begin{tabular}{p{4em}|p{7.5em}|p{16em}|p{11em}|p{7em}}
    \toprule
    Methods & Input Modalities & {Evaluation Dataset} & Data Preprocessing  & Joint Error \\
    \midrule[1.5pt]\midrule
    HuPR  & Raw signal reflections from two synchronized radars. & {Raw data: (1) More information to process, thus computationally expensive. (2) Contain rich environmental information, thus subjective to interference and domain shift.} & Tailored algorithms to obtain range-doppler-azimuth-elevation map. & MPJPE: 68 mm \\
    \midrule
    MI-Mesh & Radar PCs and cameras fusion. & {Camera: Not applicable to privacy-preserving scenarios where cameras cannot be deployed.} & Techniques to calibrate phase and handle multi-path effect. & MPJPE: 69 mm   \\
    \midrule
    mmDiff & Noisy PCs from single radar. &  {Noisy radar PCs: (1) Privacy-preserving and (2) Better cross-environment capability.} & Off-the-shelf PC generation algorithm. & MPJPE: 68 mm (mmBody) and 65 mm (mm-Fi)  \\
    \bottomrule
    \end{tabular}%

}
\caption{Qualitative Comparison with HuPR and MI-Mesh.}
\label{table:raw-compare}
\end{table}
 
\section{Supplementary Results}
\label{sec:result}

\subsection{Visualization of Diffusion Process}
As shown in Figure~\ref{diffusion}, we provide the visualization of progressive noise elimination of diffusion-based human pose estimation, where mmDiff performs progressive noise elimination and generates human poses from coarse to fine. The pose is refined from yellow to green. We can observe progressively improved keypoint accuracy during the pose refinement process: For the lab1 scene, the hands' locations are approaching the head with the increment of diffusion steps; For the rain scene, the legs' locations are also corrected to better reflect the walking poses. Meanwhile, we observe the correction of pose deformity in the smoke and dark scenes, as the shoulders' locations are progressively refined to the ground truth location. Furthermore, due to the limited pages in the main paper, we provide the visualization of motion continuity consistency and limb-length distribution of the spine length here. As shown in Figure~\ref{tempabb}, we observe the correction of erroneous frames w/ temporal motion consistency.

\subsection{Visualization of Global Radar Context}
To demonstrate the effectiveness in extracting more robust joint-wise features, we perform further visualization of the transformer's attention heatmap using the global transformer in the Global Radar Context (GRC). First, as shown in Figure~\ref{GRC3}, the global transformer extracts the self-correlation within the PC features $F^r$ and the inter-correlation between $F^r$ and $F^{j}$. In Figure~\ref{GRC4}, we further demonstrate the feature extraction of different joints does not affect each other, as they focus on different parts of the PC features. Such quality facilitates joint-wise feature extraction. Finally, in Figure~\ref{GRC1} and \ref{GRC2}, we visualize the attention region of different joint features. We observe that the feature extraction of detected joints focuses on the correct-detected PC region, which facilitates more robust feature extraction. Though feature extraction of undetected joints focuses on the wrong part, it does not affect the feature extraction of other detected joints. Therefore, the joint-wise feature extraction is more robust for detected joints.

\subsection{Visualization of Local Radar Context} 
To illustrate the effectiveness of dynamic local PC selection in the Local Radar Context (LRC), we provide a visualization of the local PC selection. We examine the local PC selection during model inference, as shown in Figure~\ref{LRC}. The dynamic joint anchors utilize intermediate diffusion poses $\hat{H}_k$, starting from coarsely estimated poses $\Tilde{H}$ (as in $k=25$) and progressively refined ($k = 25 \rightarrow 0$). Though initially, the joint anchor from $\hat{H}_k$ failed to select the upper left local PCs around the human neck, the anchor is progressively refined to the ground truth location. Finally, as $k = 0$, the upper left local PCs are considered for more robust local feature extraction. On the other hand, static joint anchors only incorporate $\Tilde{H}$, leading to biased local PC selection.

\subsection{Effect of Hyper-parameters}
\begin{table*}[ht]
\footnotesize
\centering
\caption{Parameter sensitivity analysis of the diffusion steps $K$. We record joint errors by MPJPE in white and PA-MPJPE in gray. Bold is the best and red is the worst.}
% \vspace{-1em}
% \setlength{\belowcaptionskip}{0.2cm}
\resizebox{1.\textwidth}{!}{
  \fontsize{12}{14}\selectfont
        % Table generated by Excel2LaTeX from sheet 'sense_diffusion'
    \begin{tabular}{c|cccccc|cccccccc|cc}
    \toprule
    \multicolumn{1}{c|}{\multirow{2}[2]{*}{$\textbf{K}$}} & \multicolumn{6}{c|}{\textbf{Basic Scenes}}    & \multicolumn{8}{c|}{\textbf{Adverse Environment}}             & \multicolumn{2}{c}{\multirow{2}[2]{*}{\textbf{Average}}} \\
          & \multicolumn{2}{c}{\textbf{Lab1}} & \multicolumn{2}{c}{\textbf{Lab2}} & \multicolumn{2}{c|}{\textbf{Furnished}} & \multicolumn{2}{c}{\textbf{Rain}} & \multicolumn{2}{c}{\textbf{Smoke}} & \multicolumn{2}{c}{\textbf{Poor\_lighting}} & \multicolumn{2}{c|}{\textbf{Occlusion}} & \multicolumn{2}{c}{} \\
    \midrule
    \textbf{12} & \textcolor[rgb]{ 1,  0,  0}{61.3} & \cellcolor[rgb]{ .749,  .749,  .749}\textcolor[rgb]{ 1,  0,  0}{50.23} & \textcolor[rgb]{ 1,  0,  0}{71.37} & \cellcolor[rgb]{ .749,  .749,  .749}\textcolor[rgb]{ 1,  0,  0}{66.08} & \textcolor[rgb]{ 1,  0,  0}{70.52} & \cellcolor[rgb]{ .749,  .749,  .749}\textcolor[rgb]{ 1,  0,  0}{51.76} & \textcolor[rgb]{ 1,  0,  0}{76.41} & \cellcolor[rgb]{ .749,  .749,  .749}\textcolor[rgb]{ 1,  0,  0}{60.43} & 78.75 & \cellcolor[rgb]{ .851,  .851,  .851}\textcolor[rgb]{ 1,  0,  0}{63.86} & \textcolor[rgb]{ 1,  0,  0}{67.84} & \cellcolor[rgb]{ .749,  .749,  .749}\textcolor[rgb]{ 1,  0,  0}{49.67} & \textcolor[rgb]{ 1,  0,  0}{71.22} & \cellcolor[rgb]{ .749,  .749,  .749}\textcolor[rgb]{ 1,  0,  0}{51.89} & \textcolor[rgb]{ 1,  0,  0}{71.06} & \cellcolor[rgb]{ .749,  .749,  .749}\textcolor[rgb]{ 1,  0,  0}{56.27} \\
    \textbf{25} & 59.52 & \cellcolor[rgb]{ .749,  .749,  .749}\textbf{47.85} & 69.36 & \cellcolor[rgb]{ .749,  .749,  .749}\textbf{61.23} & 67.15 & \cellcolor[rgb]{ .749,  .749,  .749}\textbf{49.19} & \textbf{71.03} & \cellcolor[rgb]{ .749,  .749,  .749}58.40 & 76.92 & \cellcolor[rgb]{ .851,  .851,  .851}\textbf{62.25} & 65.08 & \cellcolor[rgb]{ .749,  .749,  .749}\textbf{47.47} & \textbf{67.47} & \cellcolor[rgb]{ .749,  .749,  .749}49.54 & \textbf{68.08} & \cellcolor[rgb]{ .749,  .749,  .749}\textbf{53.71} \\
    \textbf{36} & \textbf{59.21} & \cellcolor[rgb]{ .749,  .749,  .749}48.68 & 69    & \cellcolor[rgb]{ .749,  .749,  .749}63.42 & 67.75 & \cellcolor[rgb]{ .749,  .749,  .749}49.79 & 72.38 & \cellcolor[rgb]{ .749,  .749,  .749}58.95 & \textbf{76.41} & \cellcolor[rgb]{ .851,  .851,  .851}62.41 & 65.54 & \cellcolor[rgb]{ .749,  .749,  .749}48.37 & 69.09 & \cellcolor[rgb]{ .749,  .749,  .749}51.12 & 68.48 & \cellcolor[rgb]{ .749,  .749,  .749}54.68 \\
    \textbf{50} & 60.16 & \cellcolor[rgb]{ .749,  .749,  .749}48.83 & \textbf{66.51} & \cellcolor[rgb]{ .749,  .749,  .749}61.39 & 67.8  & \cellcolor[rgb]{ .749,  .749,  .749}50.18 & 73.44 & \cellcolor[rgb]{ .749,  .749,  .749}\textbf{57.18} & \textcolor[rgb]{ 1,  0,  0}{80.65} & \cellcolor[rgb]{ .851,  .851,  .851}63.04 & 65.38 & \cellcolor[rgb]{ .749,  .749,  .749}48.11 & 68.11 & \cellcolor[rgb]{ .749,  .749,  .749}\textbf{49.46} & 68.86 & \cellcolor[rgb]{ .749,  .749,  .749}54.03 \\
    \textbf{60} & 59.97 & \cellcolor[rgb]{ .749,  .749,  .749}48.65 & 67.61 & \cellcolor[rgb]{ .749,  .749,  .749}62.53 & \textbf{67.07} & \cellcolor[rgb]{ .749,  .749,  .749}49.32 & 73.12 & \cellcolor[rgb]{ .749,  .749,  .749}57.37 & 80.02 & \cellcolor[rgb]{ .851,  .851,  .851}62.73 & \textbf{65.01} & \cellcolor[rgb]{ .749,  .749,  .749}47.85 & 68.34 & \cellcolor[rgb]{ .749,  .749,  .749}49.62 & 68.73 & \cellcolor[rgb]{ .749,  .749,  .749}54.01 \\
    \bottomrule
    \end{tabular}%

    }
    % \captionsetup{font=footnotesize}
    
    \label{tab:sense_K}

\end{table*}%

\begin{table*}[ht]
\footnotesize
\centering
\caption{Parameter sensitivity analysis of the $\beta$ scheduling for the diffusion model. We record joint errors by MPJPE in white and PA-MPJPE in gray. C denotes constant $\beta$ scheduling, L denotes linear $\beta$ scheduling. Bold is the best and red is the worst.}
\resizebox{1.\textwidth}{!}{
  \fontsize{12}{14}\selectfont
% Table generated by Excel2LaTeX from sheet 'sense_diffusion'
    \begin{tabular}{c|cccccc|cccccccc|cc}
    \toprule
    \multicolumn{1}{c|}{\multirow{2}[2]{*}{\textbf{\boldmath{$\beta$} scheduling}}} & \multicolumn{6}{c|}{\textbf{Basic Scenes}}    & \multicolumn{8}{c|}{\textbf{Adverse Environment}}             & \multicolumn{2}{c}{\multirow{2}[2]{*}{\textbf{Average}}} \\
          & \multicolumn{2}{c}{\textbf{Lab1}} & \multicolumn{2}{c}{\textbf{Lab2}} & \multicolumn{2}{c|}{\textbf{Furnished}} & \multicolumn{2}{c}{\textbf{Rain}} & \multicolumn{2}{c}{\textbf{Smoke}} & \multicolumn{2}{c}{\textbf{Poor\_lighting}} & \multicolumn{2}{c|}{\textbf{Occlusion}} & \multicolumn{2}{c}{} \\
    \midrule
    \textbf{C: 0.001} & \textbf{59.37} & \cellcolor[rgb]{ .749,  .749,  .749}48.66 & 67.24 & \cellcolor[rgb]{ .749,  .749,  .749}60.69 & 65.83 & \cellcolor[rgb]{ .749,  .749,  .749}48.65 & 72.24 & \cellcolor[rgb]{ .749,  .749,  .749}57.77 & 79.82 & \cellcolor[rgb]{ .851,  .851,  .851}63.55 & 64.34 & \cellcolor[rgb]{ .749,  .749,  .749}47.1 & 64.81 & \cellcolor[rgb]{ .749,  .749,  .749}48.57 & \textbf{67.66} & \cellcolor[rgb]{ .749,  .749,  .749}\textbf{53.57} \\
    \textbf{C: 0.002} & 61.29 & \cellcolor[rgb]{ .749,  .749,  .749}49.37 & 72.98 & \cellcolor[rgb]{ .749,  .749,  .749}61.7 & 66.87 & \cellcolor[rgb]{ .749,  .749,  .749}48.43 & 70.86 & \cellcolor[rgb]{ .749,  .749,  .749}57.77 & 77.47 & \cellcolor[rgb]{ .851,  .851,  .851}63.74 & 63.72 & \cellcolor[rgb]{ .749,  .749,  .749}46.76 & 71.57 & \cellcolor[rgb]{ .749,  .749,  .749}51.45 & \textcolor[rgb]{ 1,  0,  0}{69.25} & \cellcolor[rgb]{ .749,  .749,  .749}\textcolor[rgb]{ 1,  0,  0}{54.17} \\
    \textbf{L: [0.0001, 0.001]} & 59.52 & \cellcolor[rgb]{ .749,  .749,  .749}\textbf{47.85} & 69.36 & \cellcolor[rgb]{ .749,  .749,  .749}61.23 & 67.15 & \cellcolor[rgb]{ .749,  .749,  .749}49.19 & 71.03 & \cellcolor[rgb]{ .749,  .749,  .749}58.40 & 76.92 & \cellcolor[rgb]{ .851,  .851,  .851}62.25 & 65.08 & \cellcolor[rgb]{ .749,  .749,  .749}47.47 & 67.47 & \cellcolor[rgb]{ .749,  .749,  .749}49.54 & 68.08 & \cellcolor[rgb]{ .749,  .749,  .749}53.71 \\
    \textbf{L: [0.0001, 0.002]} & 60.87 & \cellcolor[rgb]{ .749,  .749,  .749}48.39 & 66.79 & \cellcolor[rgb]{ .749,  .749,  .749}61.74 & 66.66 & \cellcolor[rgb]{ .749,  .749,  .749}48.63 & 74.92 & \cellcolor[rgb]{ .749,  .749,  .749}57.88 & 80.62 & \cellcolor[rgb]{ .851,  .851,  .851}62.68 & 65.26 & \cellcolor[rgb]{ .749,  .749,  .749}47.61 & 69.45 & \cellcolor[rgb]{ .749,  .749,  .749}49.96 & 69.22 & \cellcolor[rgb]{ .749,  .749,  .749}53.84 \\
    \bottomrule
    \end{tabular}%
    }
    % \captionsetup{font=footnotesize}
    \label{tab:sense_beta}
\end{table*}%

\begin{table*}[ht]
\footnotesize
\centering
\caption{Parameter sensitivity analysis of the limb loss weighting parameter $\lambda$ for the structural limb-length consistency module. We record joint errors by MPJPE in white and PA-MPJPE in gray. Bold is the best and red is the worst.}
% \vspace{-1em}
% \setlength{\belowcaptionskip}{0.2cm}
\resizebox{1.\textwidth}{!}{
  \fontsize{12}{14}\selectfont

       % Table generated by Excel2LaTeX from sheet 'sense_diffusion'
    \begin{tabular}{c|cccccc|cccccccc|cc}
    \toprule
    \multicolumn{1}{c|}{\multirow{2}[2]{*}{\boldmath{$\lambda$}}} & \multicolumn{6}{c|}{\textbf{Basic Scenes}}    & \multicolumn{8}{c|}{\textbf{Adverse Environment}}             & \multicolumn{2}{c}{\multirow{2}[2]{*}{\textbf{Average}}} \\
          & \multicolumn{2}{c}{\textbf{Lab1}} & \multicolumn{2}{c}{\textbf{Lab2}} & \multicolumn{2}{c|}{\textbf{Furnished}} & \multicolumn{2}{c}{\textbf{Rain}} & \multicolumn{2}{c}{\textbf{Smoke}} & \multicolumn{2}{c}{\textbf{Poor\_lighting}} & \multicolumn{2}{c|}{\textbf{Occlusion}} & \multicolumn{2}{c}{} \\
    \midrule
    \textbf{2} & 59.35 & \cellcolor[rgb]{ .749,  .749,  .749}47.99 & \textbf{67.71} & \cellcolor[rgb]{ .749,  .749,  .749}61.97 & \textbf{66.99} & \cellcolor[rgb]{ .749,  .749,  .749}49.63 & \textcolor[rgb]{ 1,  0,  0}{73.04} & \cellcolor[rgb]{ .749,  .749,  .749}57.85 & \textcolor[rgb]{ 1,  0,  0}{78.77} & \cellcolor[rgb]{ .851,  .851,  .851}\textbf{62.06} & \textbf{64.99} & \cellcolor[rgb]{ .749,  .749,  .749}47.80 & 68.29 & \cellcolor[rgb]{ .749,  .749,  .749}49.70 & 68.45 & \cellcolor[rgb]{ .749,  .749,  .749}53.86 \\
    \textbf{5} & 58.65 & \cellcolor[rgb]{ .749,  .749,  .749}\textbf{47.66} & 68.91 & \cellcolor[rgb]{ .749,  .749,  .749}62.25 & \textcolor[rgb]{ 1,  0,  0}{67.86} & \cellcolor[rgb]{ .749,  .749,  .749}\textcolor[rgb]{ 1,  0,  0}{50.33} & 71.42 & \cellcolor[rgb]{ .749,  .749,  .749}\textbf{57.58} & 77.19 & \cellcolor[rgb]{ .851,  .851,  .851}62.84 & 65.50 & \cellcolor[rgb]{ .749,  .749,  .749}47.86 & 67.79 & \cellcolor[rgb]{ .749,  .749,  .749}\textbf{49.15} & 68.19 & \cellcolor[rgb]{ .749,  .749,  .749}53.95 \\
    \textbf{8} & 59.47 & \cellcolor[rgb]{ .749,  .749,  .749}\textcolor[rgb]{ 1,  0,  0}{48.47} & 68.07 & \cellcolor[rgb]{ .749,  .749,  .749}61.90 & 67.83 & \cellcolor[rgb]{ .749,  .749,  .749}49.69 & 72.34 & \cellcolor[rgb]{ .749,  .749,  .749}57.75 & 78.58 & \cellcolor[rgb]{ .851,  .851,  .851}62.72 & \textcolor[rgb]{ 1,  0,  0}{65.59} & \cellcolor[rgb]{ .749,  .749,  .749}\textcolor[rgb]{ 1,  0,  0}{48.26} & \textcolor[rgb]{ 1,  0,  0}{68.68} & \cellcolor[rgb]{ .749,  .749,  .749}\textcolor[rgb]{ 1,  0,  0}{51.25} & \textcolor[rgb]{ 1,  0,  0}{68.65} & \cellcolor[rgb]{ .749,  .749,  .749}\textcolor[rgb]{ 1,  0,  0}{54.29} \\
    \textbf{10} & \textcolor[rgb]{ 1,  0,  0}{59.52} & \cellcolor[rgb]{ .749,  .749,  .749}47.85 & \textcolor[rgb]{ 1,  0,  0}{69.36} & \cellcolor[rgb]{ .749,  .749,  .749}\textbf{61.23} & 67.15 & \cellcolor[rgb]{ .749,  .749,  .749}\textbf{49.19} & \textbf{71.03} & \cellcolor[rgb]{ .749,  .749,  .749}\textcolor[rgb]{ 1,  0,  0}{58.40} & \textbf{76.92} & \cellcolor[rgb]{ .851,  .851,  .851}62.25 & 65.08 & \cellcolor[rgb]{ .749,  .749,  .749}\textbf{47.47} & 67.47 & \cellcolor[rgb]{ .749,  .749,  .749}49.54 & 68.08 & \cellcolor[rgb]{ .749,  .749,  .749}\textbf{53.71} \\
    \textbf{15} & \textbf{58.36} & \cellcolor[rgb]{ .749,  .749,  .749}47.75 & 68.01 & \cellcolor[rgb]{ .749,  .749,  .749}\textcolor[rgb]{ 1,  0,  0}{62.65} & 67.80 & \cellcolor[rgb]{ .749,  .749,  .749}49.92 & 71.16 & \cellcolor[rgb]{ .749,  .749,  .749}57.87 & 78.22 & \cellcolor[rgb]{ .851,  .851,  .851}\textcolor[rgb]{ 1,  0,  0}{63.37} & 65.49 & \cellcolor[rgb]{ .749,  .749,  .749}47.94 & \textbf{67.00} & \cellcolor[rgb]{ .749,  .749,  .749}49.66 & \textbf{68.00} & \cellcolor[rgb]{ .749,  .749,  .749}54.17 \\
    \bottomrule
    \end{tabular}%

    }
    % \captionsetup{font=footnotesize}

    \label{tab:sense_lambda}

\end{table*}%

\begin{table*}[ht]
\footnotesize
\centering
\caption{Parameter sensitivity analysis of the historical pose sequence length $\Delta t$ for the temporal motion consistency module. We record joint errors by MPJPE in white and PA-MPJPE in gray. Bold is the best and red is the worst.}
% \vspace{-1em}
% \setlength{\belowcaptionskip}{0.2cm}
\resizebox{1.\textwidth}{!}{
  \fontsize{12}{14}\selectfont

% Table generated by Excel2LaTeX from sheet 'sense_diffusion'

    \begin{tabular}{c|cccccc|cccccccc|cc}
    \toprule
    \multicolumn{1}{c|}{\multirow{2}[2]{*}{\boldmath{$\Delta t$}}} & \multicolumn{6}{c|}{\textbf{Basic Scenes}}    & \multicolumn{8}{c|}{\textbf{Adverse Environment}}             & \multicolumn{2}{c}{\multirow{2}[2]{*}{\textbf{Average}}} \\
          & \multicolumn{2}{c}{\textbf{Lab1}} & \multicolumn{2}{c}{\textbf{Lab2}} & \multicolumn{2}{c|}{\textbf{Furnished}} & \multicolumn{2}{c}{\textbf{Rain}} & \multicolumn{2}{c}{\textbf{Smoke}} & \multicolumn{2}{c}{\textbf{Poor\_lighting}} & \multicolumn{2}{c|}{\textbf{Occlusion}} & \multicolumn{2}{c}{} \\
    \midrule
    \textbf{2} & \textcolor[rgb]{ 1,  0,  0}{60.86} & \cellcolor[rgb]{ .749,  .749,  .749}\textcolor[rgb]{ 1,  0,  0}{48.54} & 69.32 & \cellcolor[rgb]{ .749,  .749,  .749}62.82 & 67.72 & \cellcolor[rgb]{ .749,  .749,  .749}49.68 & 72.94 & \cellcolor[rgb]{ .749,  .749,  .749}57.85 & \textcolor[rgb]{ 1,  0,  0}{81.39} & \cellcolor[rgb]{ .851,  .851,  .851}\textcolor[rgb]{ 1,  0,  0}{63.72} & 65.19 & \cellcolor[rgb]{ .749,  .749,  .749}48.18 & \textcolor[rgb]{ 1,  0,  0}{69.25} & \cellcolor[rgb]{ .749,  .749,  .749}\textcolor[rgb]{ 1,  0,  0}{50.99} & \textcolor[rgb]{ 1,  0,  0}{69.52} & \cellcolor[rgb]{ .749,  .749,  .749}\textcolor[rgb]{ 1,  0,  0}{54.54} \\
    \textbf{4} & 59.59 & \cellcolor[rgb]{ .749,  .749,  .749}47.77 & 68.63 & \cellcolor[rgb]{ .749,  .749,  .749}62.75 & 67.11 & \cellcolor[rgb]{ .749,  .749,  .749}49.45 & 73.05 & \cellcolor[rgb]{ .749,  .749,  .749}57.59 & 79.91 & \cellcolor[rgb]{ .851,  .851,  .851}63.12 & 65.50 & \cellcolor[rgb]{ .749,  .749,  .749}47.93 & 68.70 & \cellcolor[rgb]{ .749,  .749,  .749}49.80 & 68.93 & \cellcolor[rgb]{ .749,  .749,  .749}54.06 \\
    \textbf{6} & 59.52 & \cellcolor[rgb]{ .749,  .749,  .749}47.85 & \textcolor[rgb]{ 1,  0,  0}{69.36} & \cellcolor[rgb]{ .749,  .749,  .749}\textbf{61.23} & 67.15 & \cellcolor[rgb]{ .749,  .749,  .749}49.19 & \textbf{71.03} & \cellcolor[rgb]{ .749,  .749,  .749}58.40 & \textbf{76.92} & \cellcolor[rgb]{ .851,  .851,  .851}62.25 & 65.08 & \cellcolor[rgb]{ .749,  .749,  .749}47.47 & 67.47 & \cellcolor[rgb]{ .749,  .749,  .749}49.54 & \textbf{68.08} & \cellcolor[rgb]{ .749,  .749,  .749}53.71 \\
    \textbf{8} & \textbf{58.44} & \cellcolor[rgb]{ .749,  .749,  .749}47.89 & 68.79 & \cellcolor[rgb]{ .749,  .749,  .749}\textcolor[rgb]{ 1,  0,  0}{64.02} & \textcolor[rgb]{ 1,  0,  0}{68.00} & \cellcolor[rgb]{ .749,  .749,  .749}\textcolor[rgb]{ 1,  0,  0}{50.44} & 72.15 & \cellcolor[rgb]{ .749,  .749,  .749}\textcolor[rgb]{ 1,  0,  0}{58.52} & 77.18 & \cellcolor[rgb]{ .851,  .851,  .851}\textbf{61.81} & \textcolor[rgb]{ 1,  0,  0}{65.86} & \cellcolor[rgb]{ .749,  .749,  .749}\textcolor[rgb]{ 1,  0,  0}{48.58} & \textbf{67.12} & \cellcolor[rgb]{ .749,  .749,  .749}50.19 & 68.22 & \cellcolor[rgb]{ .749,  .749,  .749}54.49 \\
    \textbf{10} & 58.57 & \cellcolor[rgb]{ .749,  .749,  .749}\textbf{47.51} & \textbf{68.05} & \cellcolor[rgb]{ .749,  .749,  .749}62.59 & \textbf{66.96} & \cellcolor[rgb]{ .749,  .749,  .749}\textbf{49.01} & \textcolor[rgb]{ 1,  0,  0}{73.10} & \cellcolor[rgb]{ .749,  .749,  .749}\textbf{57.47} & 78.14 & \cellcolor[rgb]{ .851,  .851,  .851}62.46 & \textbf{64.90} & \cellcolor[rgb]{ .749,  .749,  .749}\textbf{47.34} & 67.74 & \cellcolor[rgb]{ .749,  .749,  .749}\textbf{49.23} & 68.21 & \cellcolor[rgb]{ .749,  .749,  .749}\textbf{53.66} \\
    \bottomrule
    \end{tabular}%

    }
    % \captionsetup{font=footnotesize}
    \label{tab:sense_t}

\end{table*}%

\subsubsection{Effect of diffusion steps \boldmath{$K$}.} As shown in Table~\ref{tab:sense_K}, we present how the joint error is affected by the number of diffusion steps $K$ on mmBody~\cite{chen2022mmbody}. When diffusion steps $K < 25$, we observe that the increment of $K$ can improve the performance of mmDiff. As with more iterations, mmDiff potentially can handle noisier human poses. However, with the number of diffusion steps $K > 25$, the performance of mmDiff converges. We argue that the pose noise within the coarsely estimated human poses is well handled with 25 diffusion steps. 

\subsubsection{Effect of \boldmath{$\beta$} scheduling.} As shown in Table~\ref{tab:sense_beta}, we present how the $\beta$ scheduling affects the diffusion-based HPE. We observe different $\beta$ scheduling significantly affects the mmDiff performance, as the selected noise scale should accurately approximate the noise contained by the coarsely estimated human poses. For linear scheduling, if the $\beta$ range is increased (as in range$[0.0001, 0.002]$), the performance drops significantly as the reverse diffusion process is not stable. We also observe that constant $\beta$ scheduling also performs well, as long as the noise scale is selected properly.

\subsubsection{Effect of the weighting parameter \boldmath{$\lambda$} for \boldmath{$\mathcal{L}_{\text {diff}}$}.} As shown in Table~\ref{tab:sense_lambda}, we present how the model performs with different weighting parameters $\lambda$ to integrate the limb loss $\left|L-\hat{L}\right|$ into the diffusion loss $\mathcal{L}_{\text {diff}}$. We observe that our model is not sensitive to the selection of $\lambda$, with $68.27 \pm 0.24$ (MPJPE) statistically lower than the performance without spatial limb consistency, 69.16 (MPJPE). We argue that as long as the limb loss is presented, the model can estimate a subject's limb length with acceptable accuracy. 

\subsubsection{Effect of the sequence length \boldmath{$\Delta t$}.} As shown in Table~\ref{tab:sense_t}, we present how our approach is affected by the number of adjacent time frames used in the temporal motion consistency module. When the sequence length $\Delta t \leq 6$, we observe that the increment of $\Delta t$ can improve the performance. As with longer sequence lengths, mmDiff potentially can extract more reliable and robust motion patterns of the subjects. However, as the sequence lengths $K > 6$ keep increasing, the performance of mmDiff begins to drop, especially in adverse environments. As the training of mmBody is conducted on basic scenes, the increment of sequence length tends to overfit the model to basic scenes, causing a performance drop in adverse environments. As a result, $\Delta t = 6$ is the optimum for the mmBody dataset.

\begin{figure*}[!t]
\centering
\includegraphics[width=1.\linewidth]{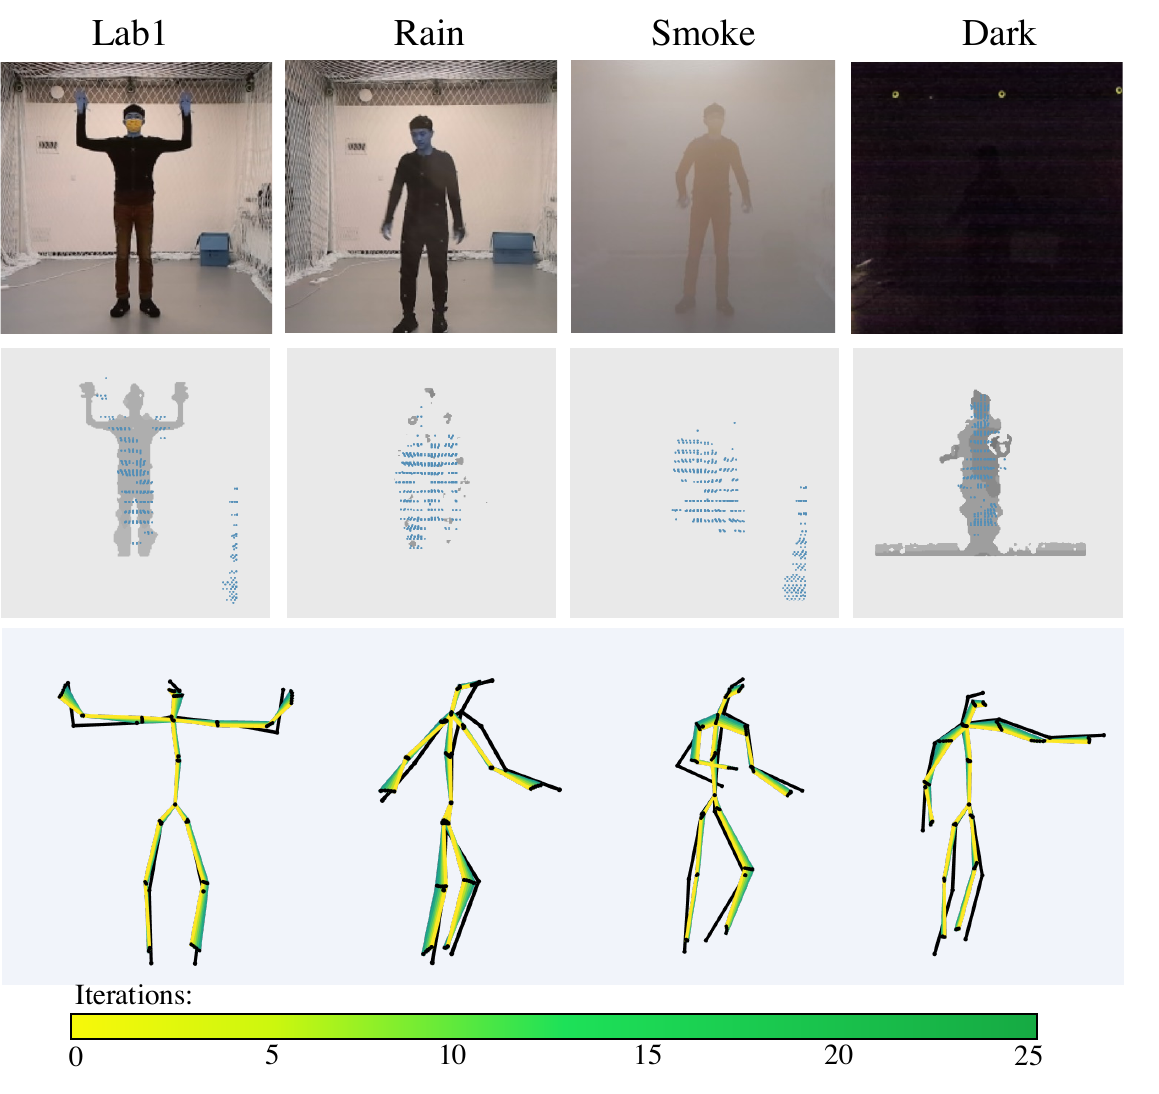}
\caption{Visualization of diffusion-based human pose estimation with diffusion 25 steps. We use gradient colors (from yellow to green) to illustrate the refined poses of different iterations. The yellow pose is the initialized coarse human pose, and the green pose is the final refined pose.}
\label{diffusion}
\end{figure*}

\begin{figure*}[!t]
\centering
\includegraphics[width=1.\linewidth]{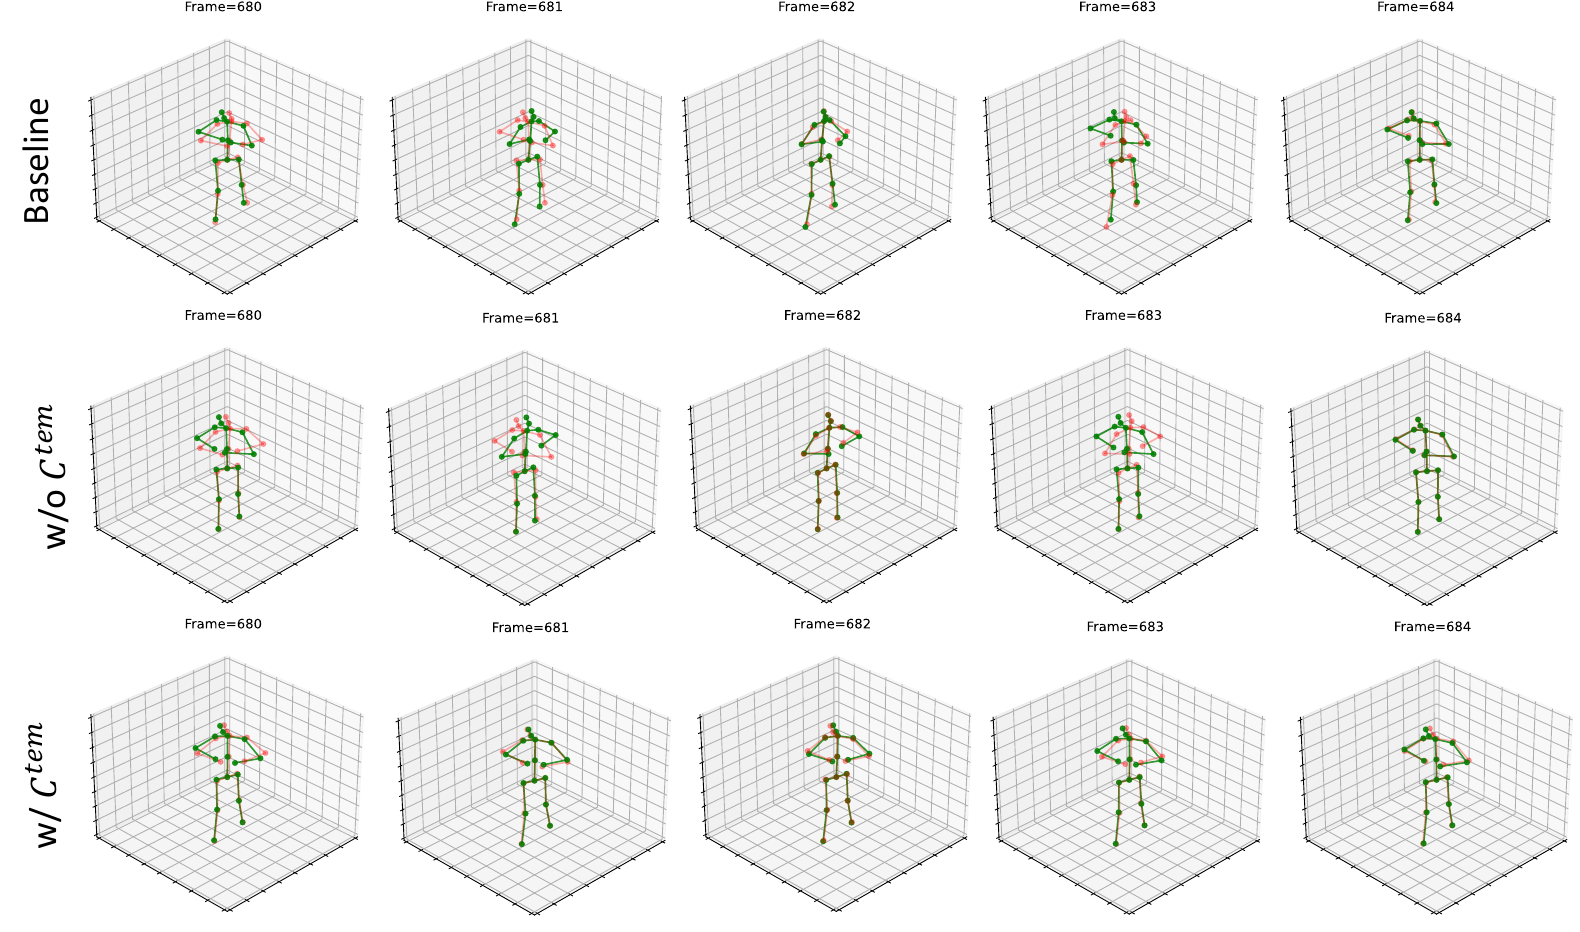}
\caption{Visualization of motion continuity on mm-Fi, with PointTransformer baseline~\cite{zhao2021point}, ours w/o $C^{tem}$ and ours w/ $C^{tem}$. Green poses are the ground truth and red poses are the prediction. We can observe occasion erroneous frames are corrected based on smooth motion patterns.}
\label{tempabb}
\end{figure*}

\begin{figure*}[!t]
\centering
\includegraphics[width=1.\linewidth]{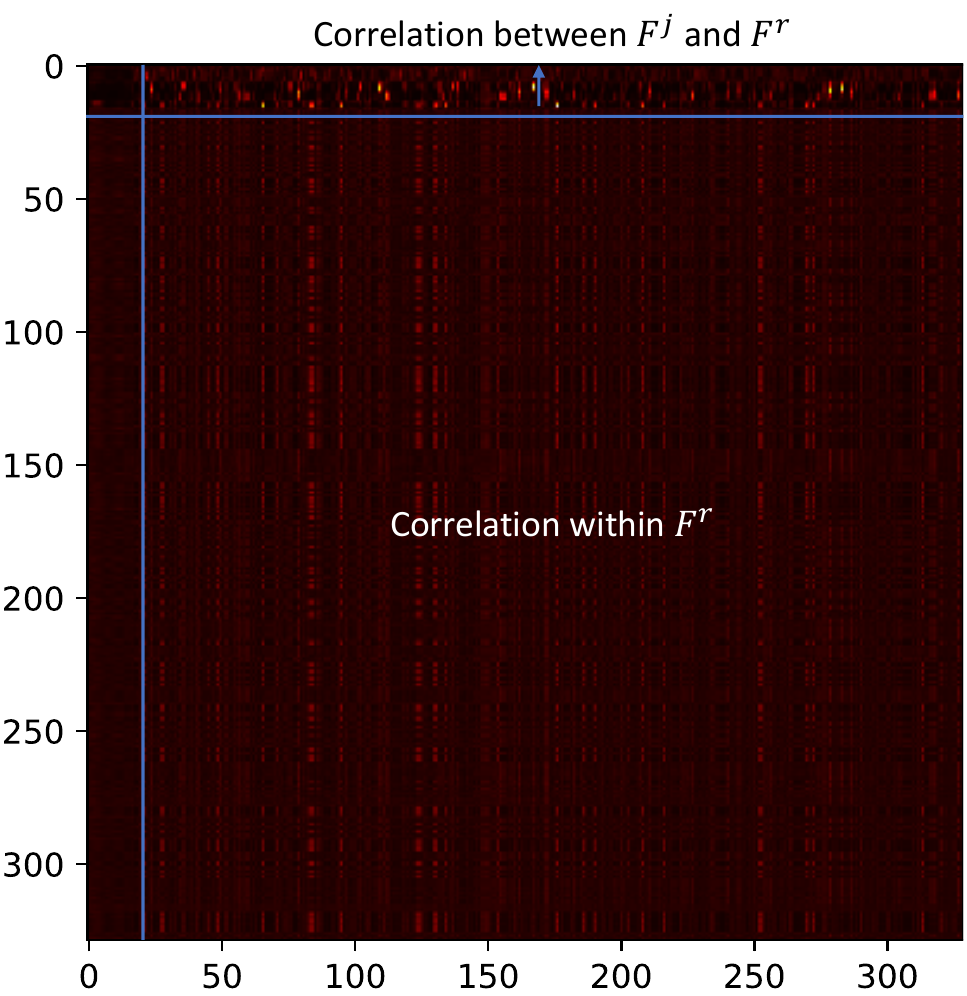}
\caption{Visualization of the correlation using the global transformer $\phi^g$ of GRC tested on mmBody: within PC features $F^r$, and between joint features $F^j$ and PC features $F^{r}$.}
\label{GRC3}
\end{figure*}

\begin{figure*}[!t]
\centering
\includegraphics[width=1.\linewidth]{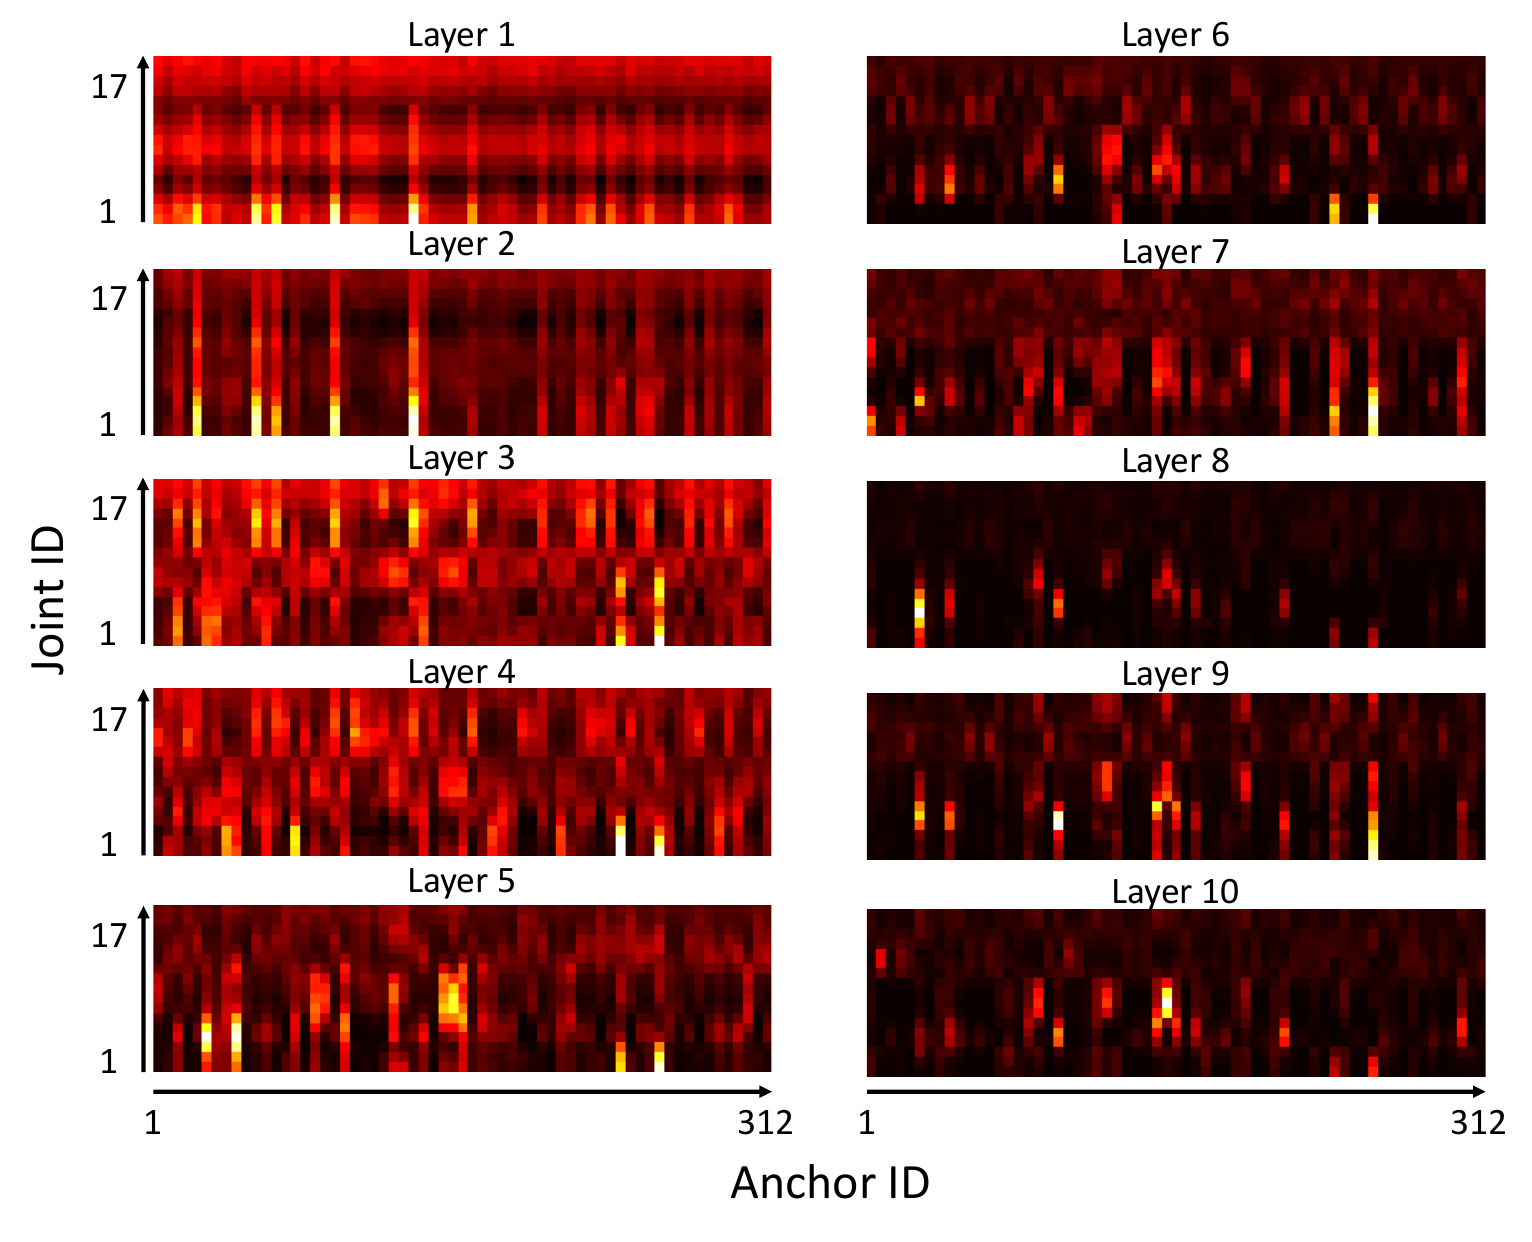}
\caption{Visualization of the correlation between joint features $F^j$ and PC features $F^{r}$, using the global transformer $\phi^g$ of GRC tested on mmBody. Feature extraction of different joints depends on individual correlation with the PC feature, which is less affected by other joint features after 5 transformer layers.}
\label{GRC4}
\end{figure*}

\begin{figure*}[!t]
\centering
\includegraphics[width=1.\linewidth]{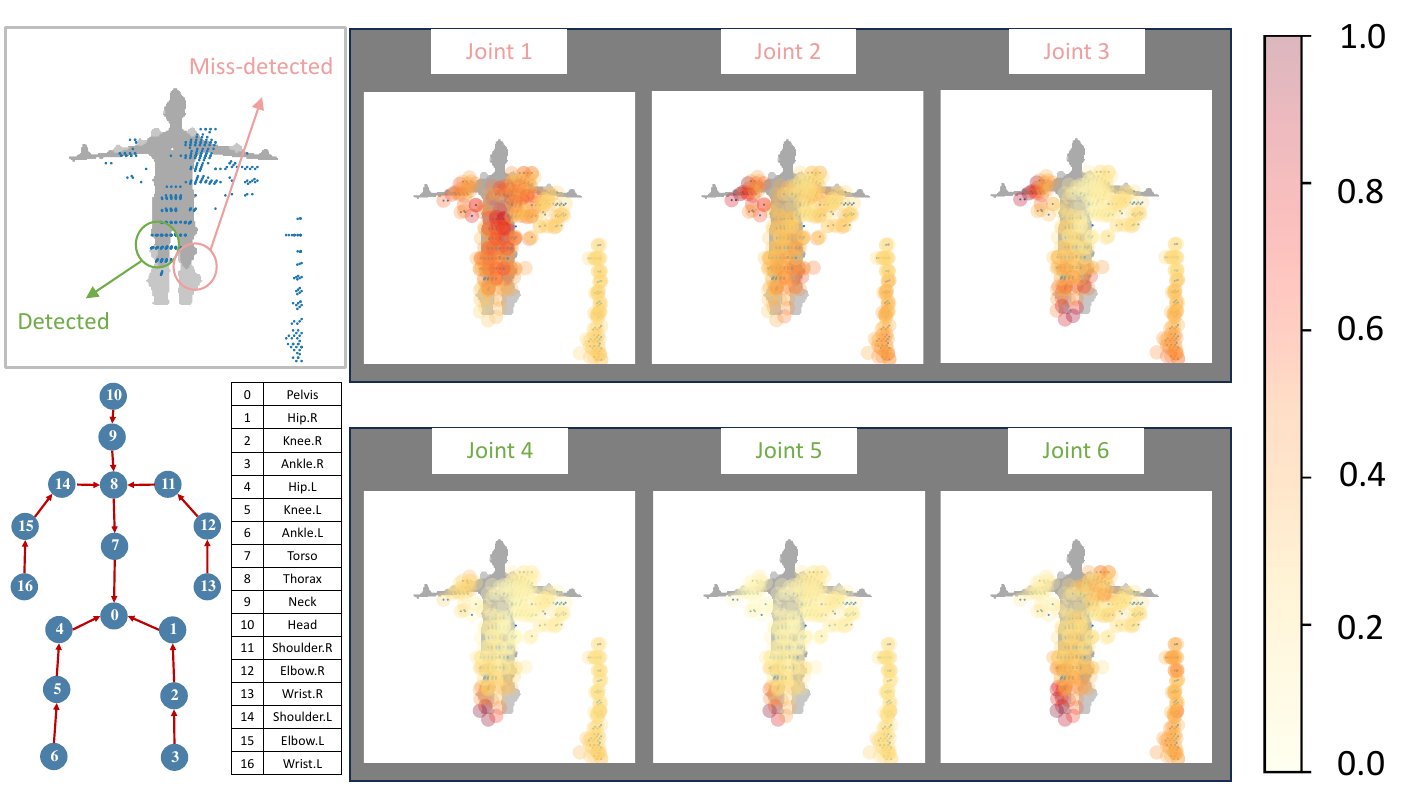}
\caption{Visualization of the attention when performing feature extraction of joints 1-6 (legs). Each joint performs individual feature extraction. For detected joints 4-6(left leg), the attention is more concentrated as correctly focuses on the left leg part, extracting more robust features. The feature extraction is more distracted and less reliable for undetected joints 1-3 (right leg) due to miss-detection.}
\label{GRC1}
\end{figure*}

\begin{figure*}[!t]
\centering
\includegraphics[width=1.\linewidth]{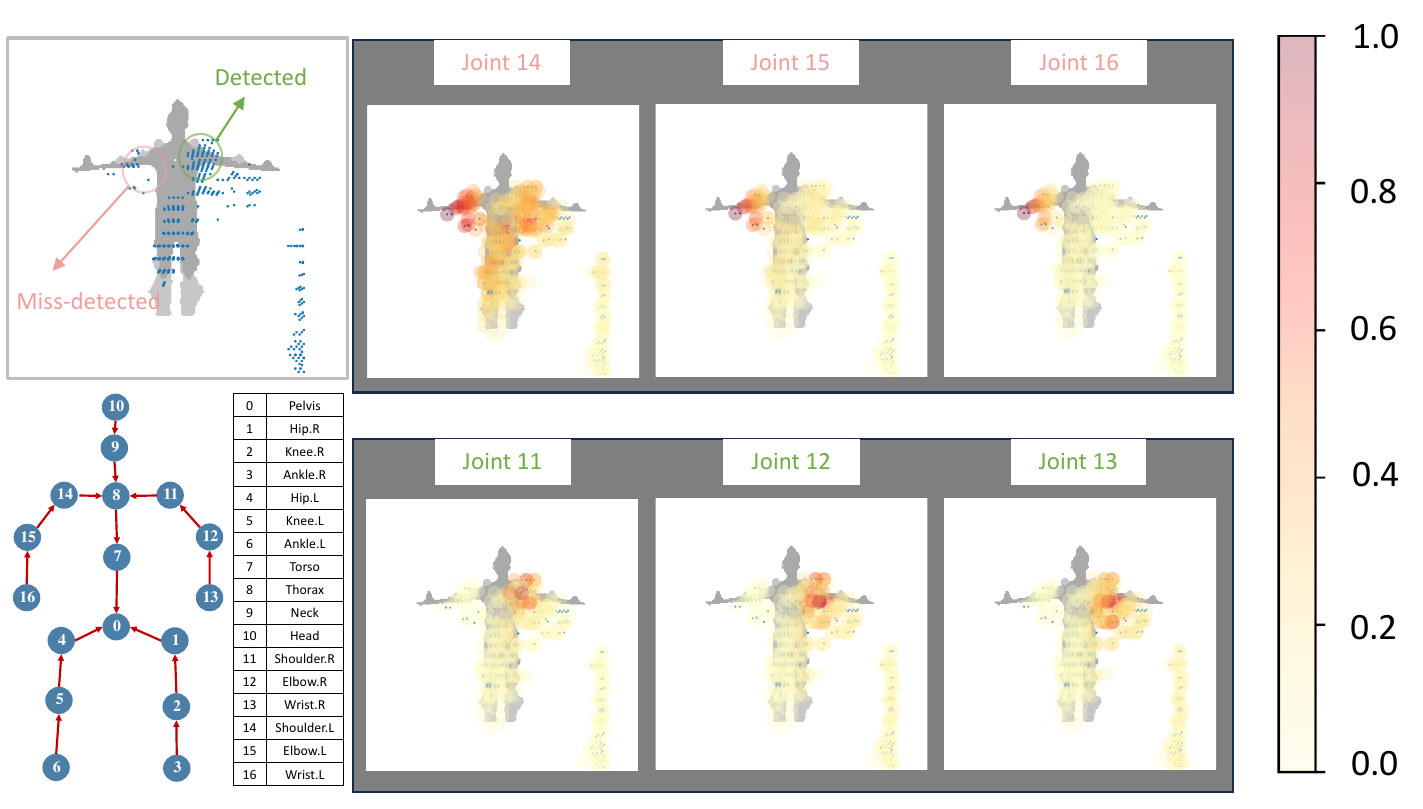}
\caption{Visualization of the attention when performing feature extraction of joints 11-16 (arms). As reflected by the attention heatmap, detected joints 11-13(right arm) have more robust features, preventing the influence of undetected joints 14-16 (left arm).}
\label{GRC2}
\end{figure*}

\begin{figure*}[!t]
\centering
\includegraphics[width=1.\linewidth]{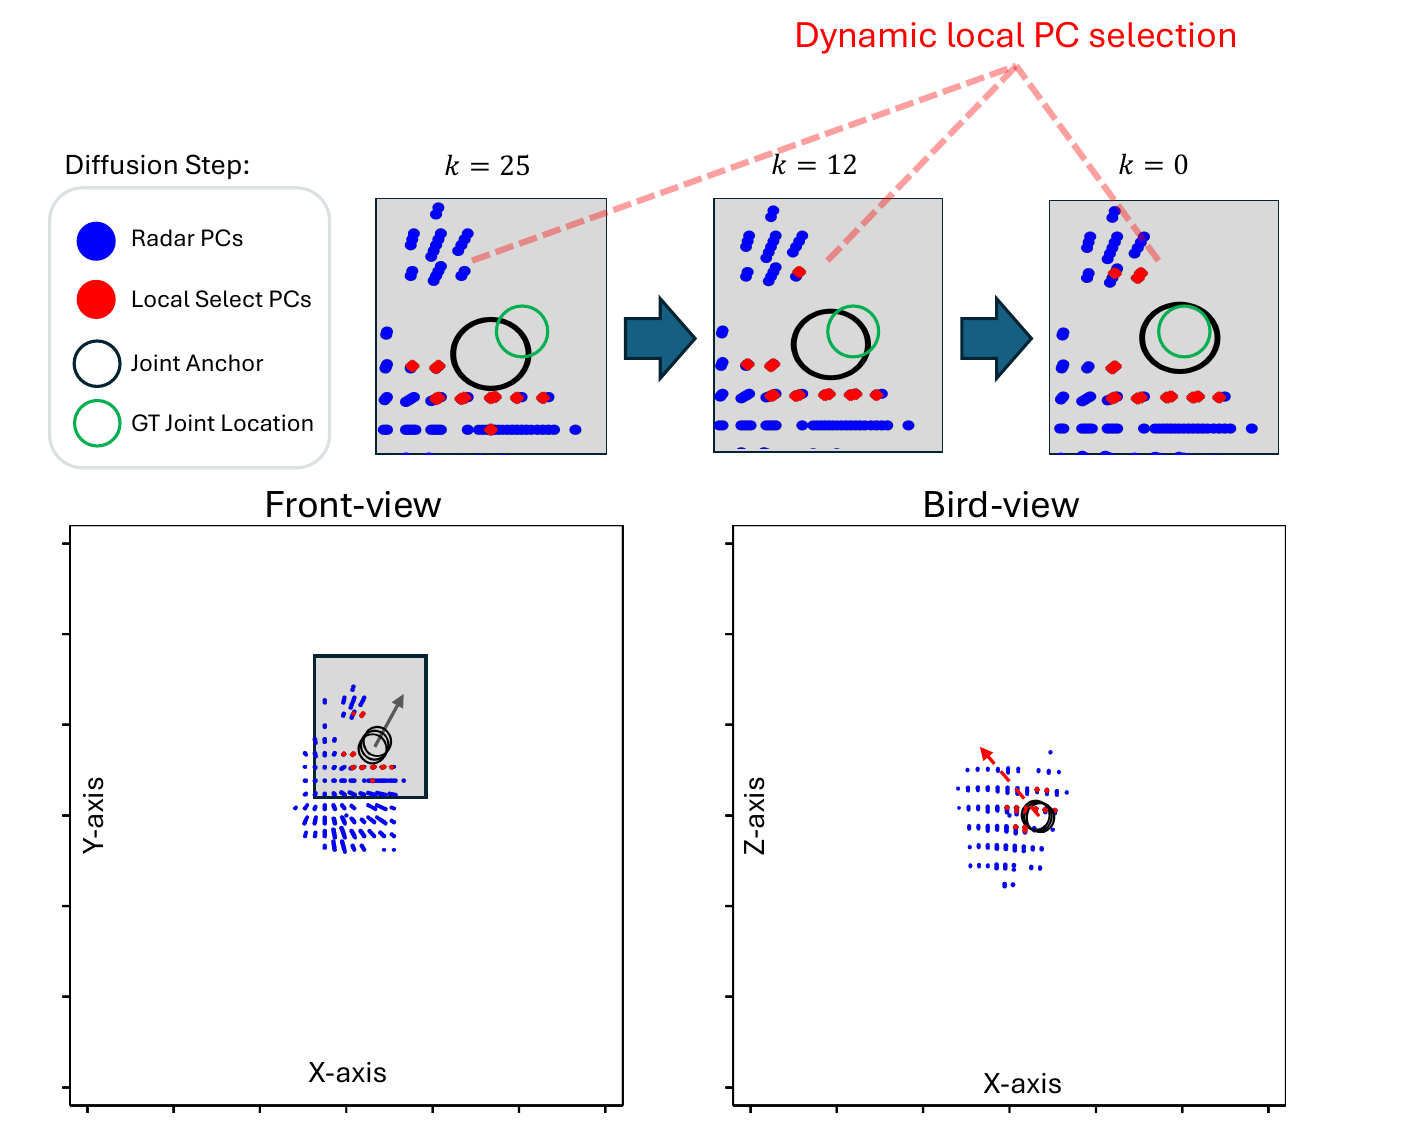}
\caption{Visualization of the local PC selection using dynamic joint anchors (right shoulder) during model inference phase. Initially, as $k = 25$, the joint anchor is derived from the coarsely estimated pose $\Tilde{H}$, failing to select the upper left local PCs. The dynamic joint-anchor starts from $\Tilde{H}$ and is progressively refined with the diffusion steps $k = 25 \rightarrow 0$. Finally, as $k = 0$, the upper left local PCs are selected for more robust local PC features. As the upper left PCs correspond to the human neck, a more robust local feature is extracted considering both shoulder and neck PCs.}
\label{LRC}
\end{figure*}

% \small
% \bibliographystyle{ieeenat_fullname}
% \bibliography{main}
